# Supplementary material for: Outlier-Based Domain of Applicability Identification for Materials Property Prediction Models
Source: arXiv:2302.06454 ancillary file (2023-01-17)
Supplement: Supplementary file 1 [file Supporting_Information.pdf]

# Supporting Information: Outlier-Based Domain of Applicability Identification for Materials Property Prediction Models

Gihan Panapitiya* and Emily Saldanha

E-mail: gihan.panapitiya@pnnl.gov

## Data

Our solubility dataset is composed using three prior datasets: PNNL Organic Solubility dataset, AqSolDB[1] and Cui dataset.[2] Our data processing pipleline is shown in Figure S1. The three datasets are first merged. The smiles common to PNNL and Cui datasets are removed from the Cui set (This is a strange step. I did this because I found PNNL data are more trustworthy than the Cui data. But, probably, we should've done a simple merge). Next, we find the duplicated SMILES. If the number of duplicates is two, we check whether the logS difference between the corresponding two molecules is less than a threshold. If the difference is less than a threshold, we keep one of them in the dataset (the other option is to use the average of the two) If the difference is greater than the threshold, we check whether the solubilities of any of these molecules are available in the PubChem dataset. If the difference between the solubility values in our current databse and those found from PubChem is greater than a threshold, we discard them. From of the remaining molecules, we check whether we still have duplicates. If so, we check if the difference between the logS values of the duplicates is less than a threshold and use the average logS as the logS of the

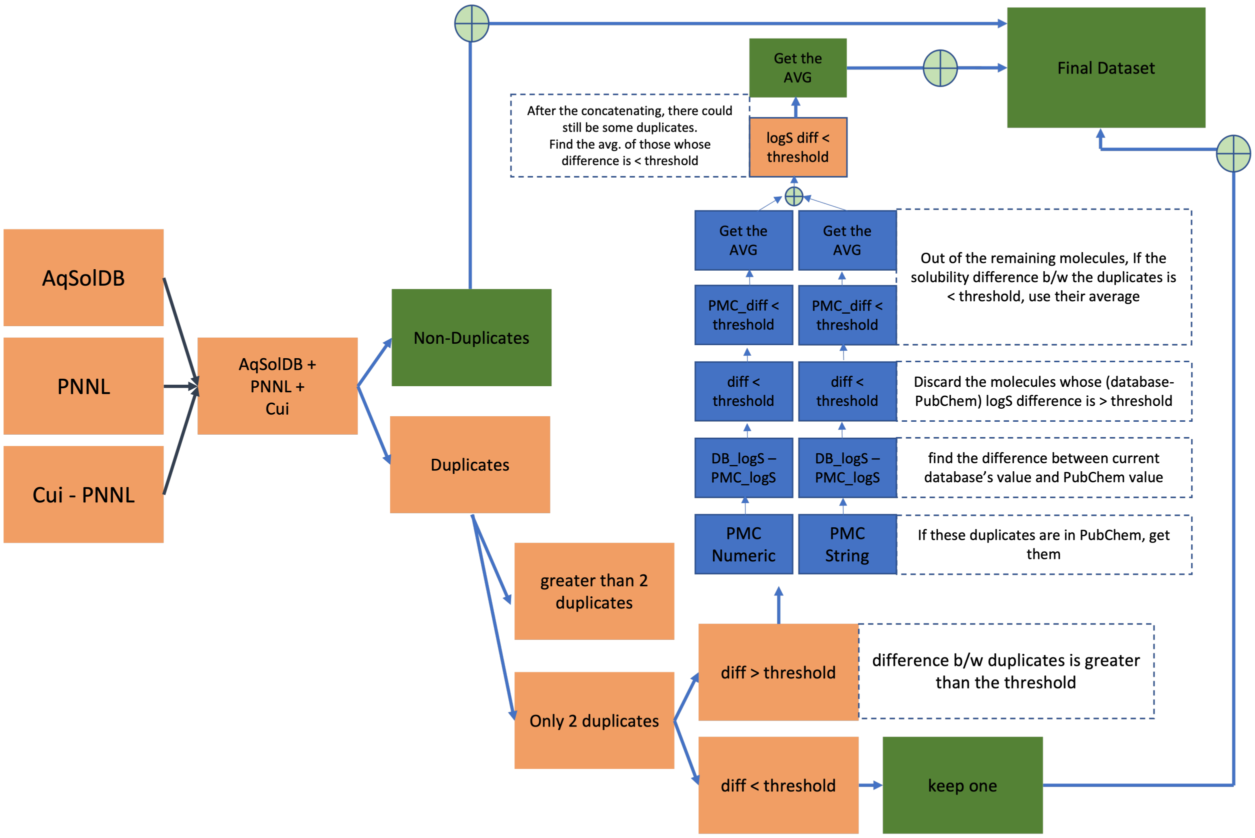


Figure S1: Data collection pipeline

duplicated SMILES. Next, we concatenate deduplicated SMILES from PubChem numeric and string sources. It is possible that after the concatenation, we still get some duplicates. In that case, as the final logS, we use the average solubility of the duplicates whose solubility difference is less than a threshold.

# KMeans clsutering

KMeans algorithm was run 10 times with different random seeds. At each time, elbow method implemented in the YellowBricks was used to find the optimal number of clusters. For the elbow method, the number of clusters was varied from 4 to 30. After finding the optimal number of clusters, KMeans was run using the same random seed used in the elbow method to find the cluster labels of the molecules in the dataset being considered. This process results in 10 sets of cluster labels for each molecule. We then find the molecules that

Table S1: Definitions of the descriptors in Table 1 in the main text. These definitions are from the reference Moriwaki et al.[3] and Panapitiya et al.[4]

| Descriptor | Description |
|---|---|
| NssssSn | Number of ssssSn[3] |
| Mpe | mean of constitutional weighted by pauling EN[3] |
| IC2 | 2-ordered neighborhood information content[3] |
| n10AHRing | 10-membered aromatic hetero ring count[3] |
| IC3 | 3-ordered neighborhood information content[3] |
| bpol | bond polarizability[3] |
| n5FRing | 5-membered fused ring count[3] |
| nFRing | fused ring count[3] |
| SsssNH | sum of sssNH[3] |
| nG12aHRing | 12-or-greater-membered[3] aromatic hetero ring count[3] |
| TIC5 | 5-ordered neighborhood total information content[3] |
| ATSC0v | centered moreau-broto autocorrelation of lag 0 weighted by vdw volume[3] |
| SsAsH2 | sum of sAsH2[3] |
| n5 | Number of atoms in the 5th concentric layer around the centroid of the molecule; 9 and 11 angstroms away from the centroid.[4] |
| nG12AHRing | 12-or-greater-membered aromatic hetero ring count[3] |
| ATS1m | a moreau-broto autocorrelation of lag 1 weighted by mass[3] |
| fMF | molecular framework ratio[3] |
| nRing | ring count[3] |
| ATS2m | moreau-broto autocorrelation of lag 2 weighted by mass[3] |
| ATS0p | moreau-broto autocorrelation of lag 0 weighted by polarizability[3] |

gets clustered together more 85% of the time. Only the molecules that satisfy this criteria were considered for the final clusters.

# Unsupervised Anomaly Detection

Each anomaly detector is fit using the standard scaled data. Probability of each data point being an outlier is found using the predict_proba method in pyod methods. First and second values in the probability list are the predition probabilities for inlier and outlier. Confidence of the prediction is also returned. Then the prediction is made by finding the class of the maximum probability. We only use predictions that have been made with confidence >= 0.99. Out of those, we select the ones got classified as outliers. As the final outliers, we only select the ones which have been predicted as outlier by at least 2 detection methods.

# Complexities of PNNL, Cui and Delaney datasets

Table provides the definitions of the molecular descriptors found in the main text.

Table S2: Selected structural properties of different datasets to show the dataset diversity. N: number of molecules, logS: log solubility, Atoms: number of atoms, AromAtom: Number of aromatic atoms, Rings: number of rings, Mass: molecular mass, HeavyAtom: number of heavy atoms, AromBond: number of aromatic bonds.

| Dataset | N | logS | Atoms | AromAtom | Rings | Mass | HeavyAtom | AromBond |
|---|---|---|---|---|---|---|---|---|
| PNNL | 20229 | -17.5 - 2.0 | 1 - 670 | 0 - 206 | 0 - 36 | 9 - 5295 | 1 - 388 | 0 - 208 |
| Cui | 9933 | -18.2 - 1.7 | 1 - 216 | 0 - 60 | 0 - 16 | 16 - 1582 | 1 - 109 | 0 - 64 |
| Delaney | 1117 | -9.7 - 1.1 | 4 - 119 | 0 - 28 | 0 - 8 | 16 - 780 | 1 - 55 | 0 - 30 |

Table S3: Definitions of the descriptors in Figure 5 and 9. These definitions are from the reference Moriwaki et al.[3]

| Descriptor | Description |
|---|---|
| nI | Number of Iodine atoms |
| MW | Molecular weight |
| AMW | averaged exact molecular weight |
| nX | number of halogen atoms |
| nBr | number of Br atoms |
| nRot | Number of rotational bonds |
| nBonds | number of all bonds in non-kekulized structure |
| C2SP3 | Number of SP3 hybridized carbons bonded to two other carbon atoms |
| nBondsS | number of single bonds in non-kekulized structure |
| nAtom | Number of atoms |
| apol | atomic polarizability |
| nBase | basic group count |
| nAcid | acidic group count |
| VMcGowan | McGowan volume |
| nBondsKD | number of double bonds in kekulized structure |
| BertzCT | a descriptor designed to quantify “complexity” of molecules |
| nBondsM | number of multiple bonds in non-kekulized structure |
| nBondsA | number of aromatic bonds in non-kekulized structure |
| nBondsO | number of bonds connecting to heavy atom in non-kekulized structure |
| nH | number of H atoms |
| nBondsKS | number of single bonds in kekulized structure |
| C3SP3 | SP3 carbon bound to 3 other carbons |
| nG12HRing | 12-or-greater-membered hetero ring count |
| nAtom | number of all atoms |
| MW | exact molecular weight |
| nHetero | number of hetero atoms |
| bpol | bond polarizability |
| C1SP3 | SP3 carbon bound to 1 other carbon |
| nP | number of P atoms |
| nS | number of S atoms |
| nF | number of F atoms |
| nHeavyAtom | number of heavy atoms |
| nCl | number of Cl atoms |
| fragCpx | fragment complexity |
| FilterItLogS | A theoretical approximation for logS by Filter-it$^{TM}$ |
| nN | number of N atoms |
| nC | number of C atoms |
| TopoPSA | topological polar surface area |
| TopoPSA(NO) | topological polar surface area (use only nitrogen and oxygen) |

## More examples of subdomains

Here, we present more examples for the subdomains disucssed in the section 3.3 of the main text.

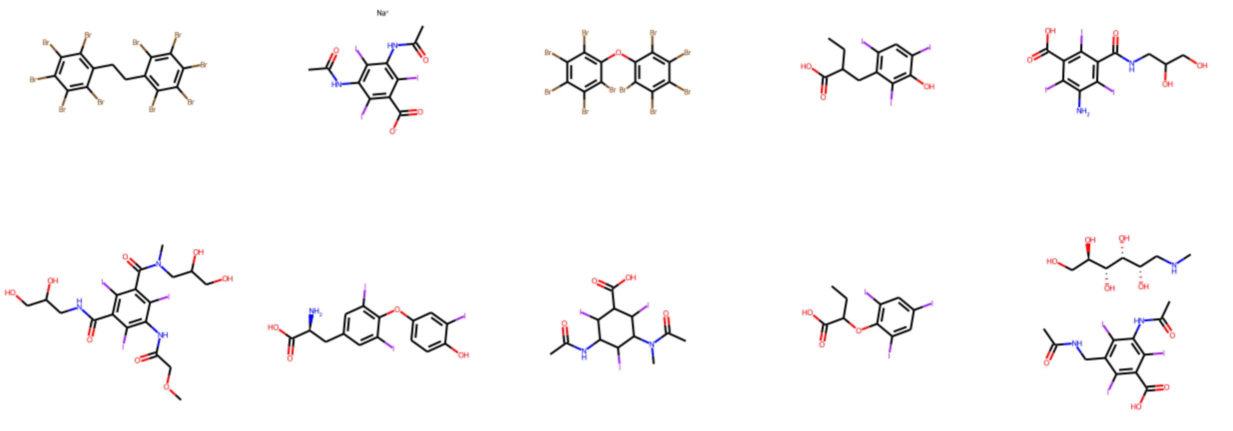

(a) Group 1

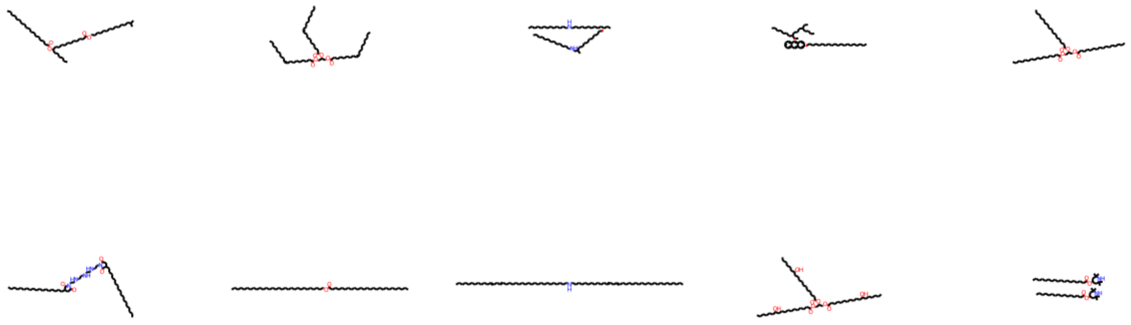

(b) Group 2

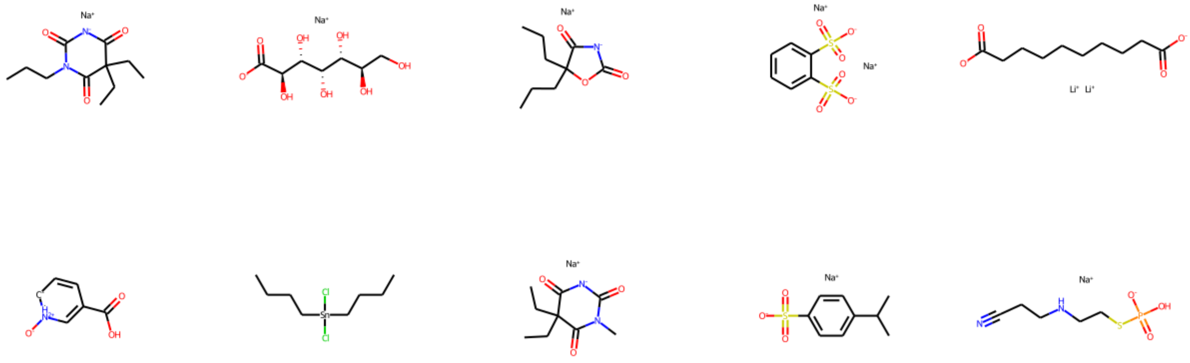

(c) Group 3

Figure S2: Examples for groups 1,2 and 3.

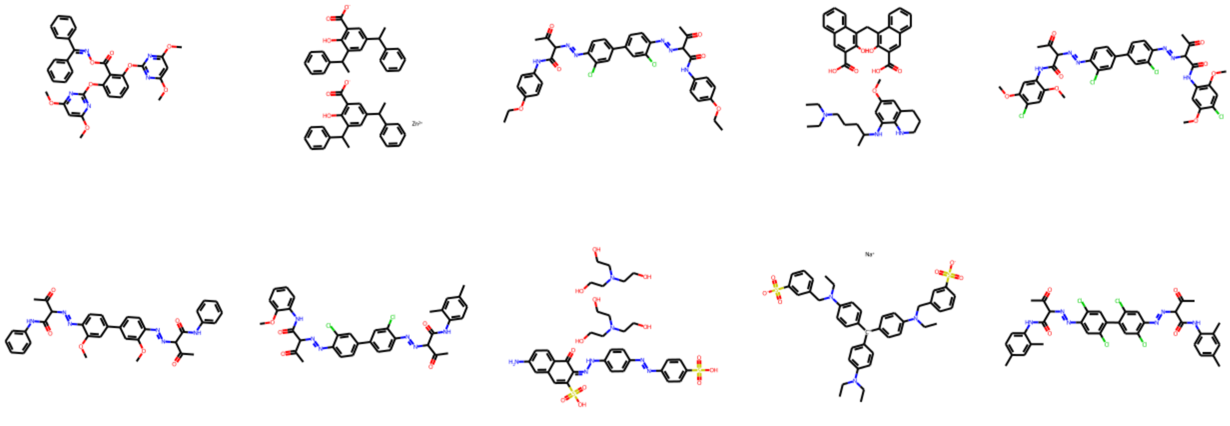

(a) Group 4

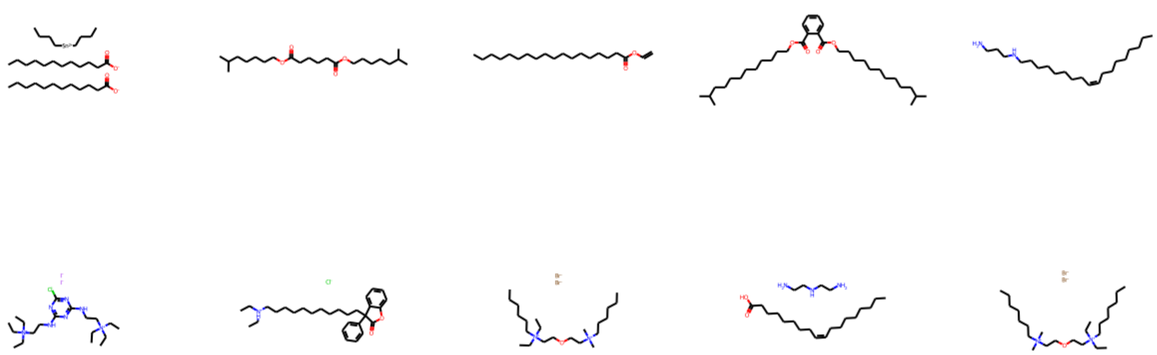

(b) Group 5

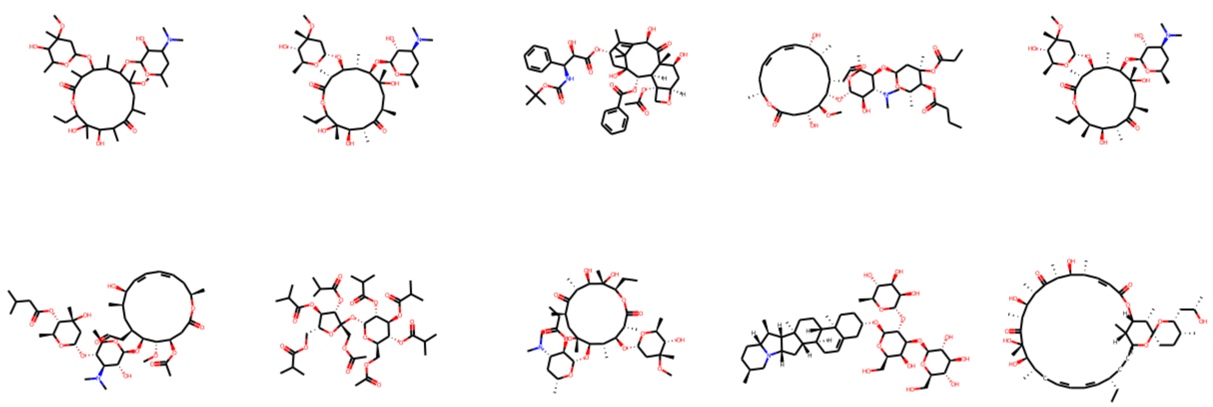

(c) Group 6

Figure S3: Examples for groups 4,5 and 6.

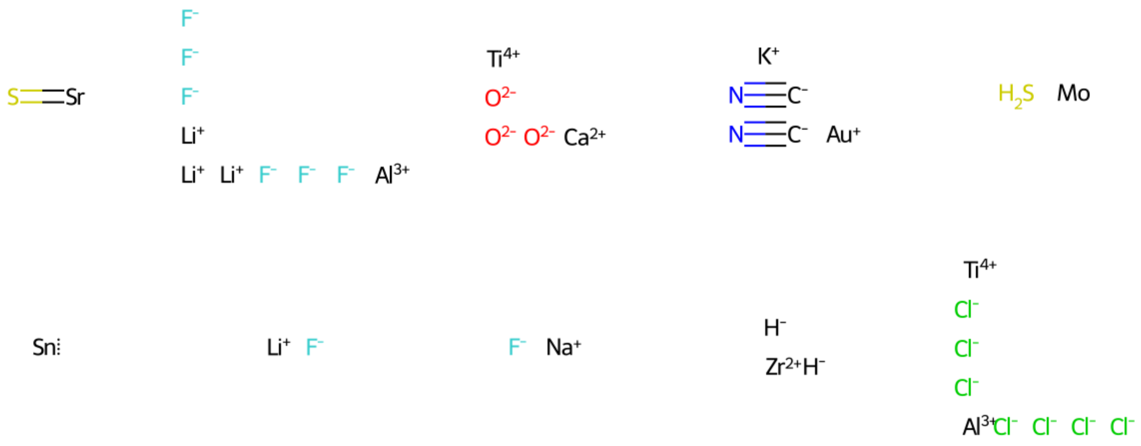


(a) Group 7

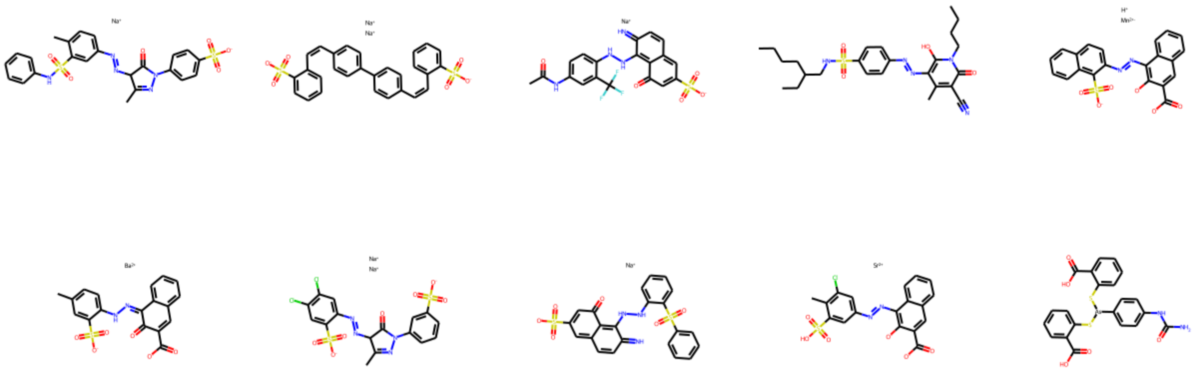

(b) Group 8

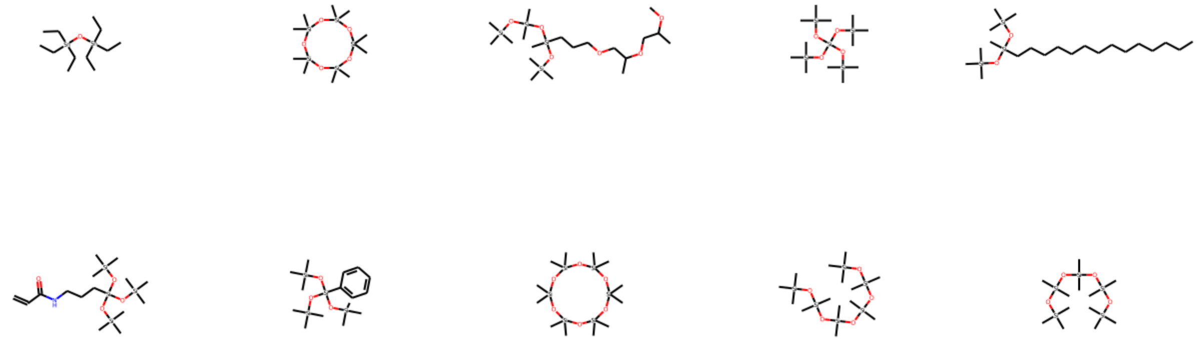

(c) Group 9

Figure S4: Examples for groups 7,8 and 9.

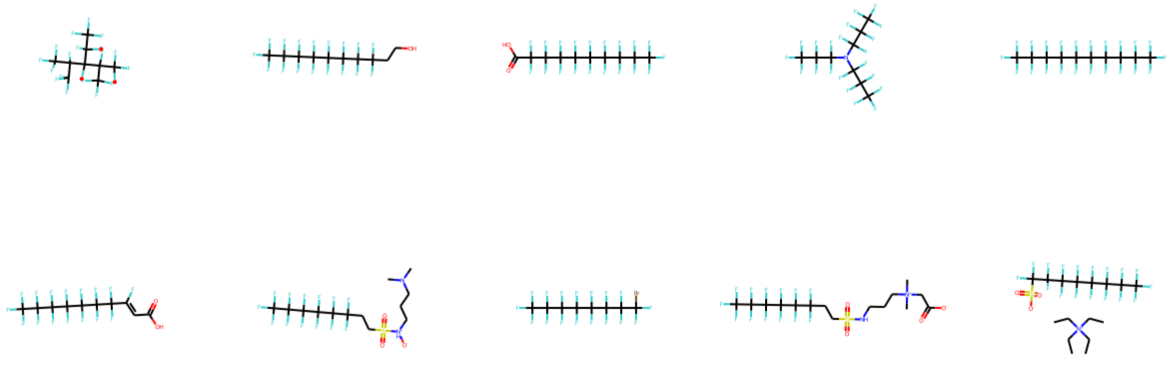

(a) Group 10

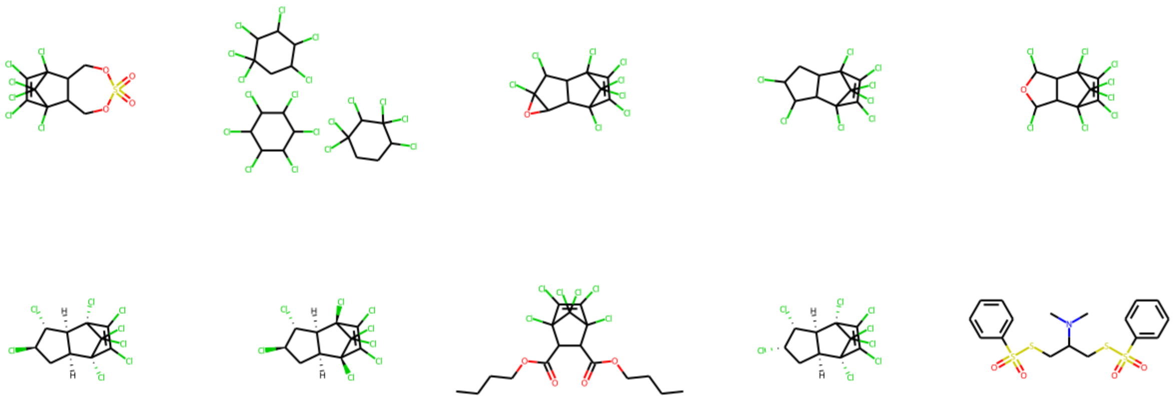

(b) Group 11

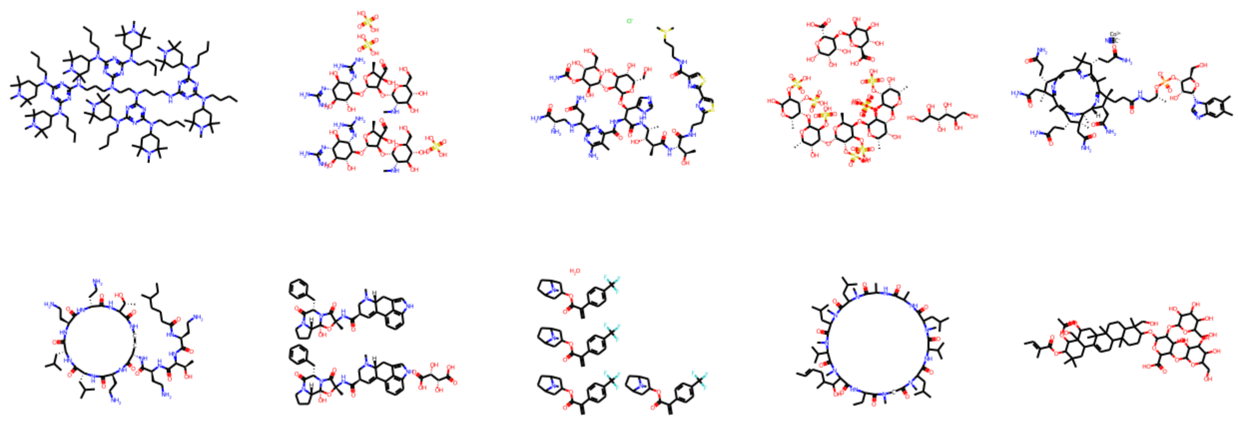

(c) Group 12

Figure S5: Examples for groups 10,11 and 12.

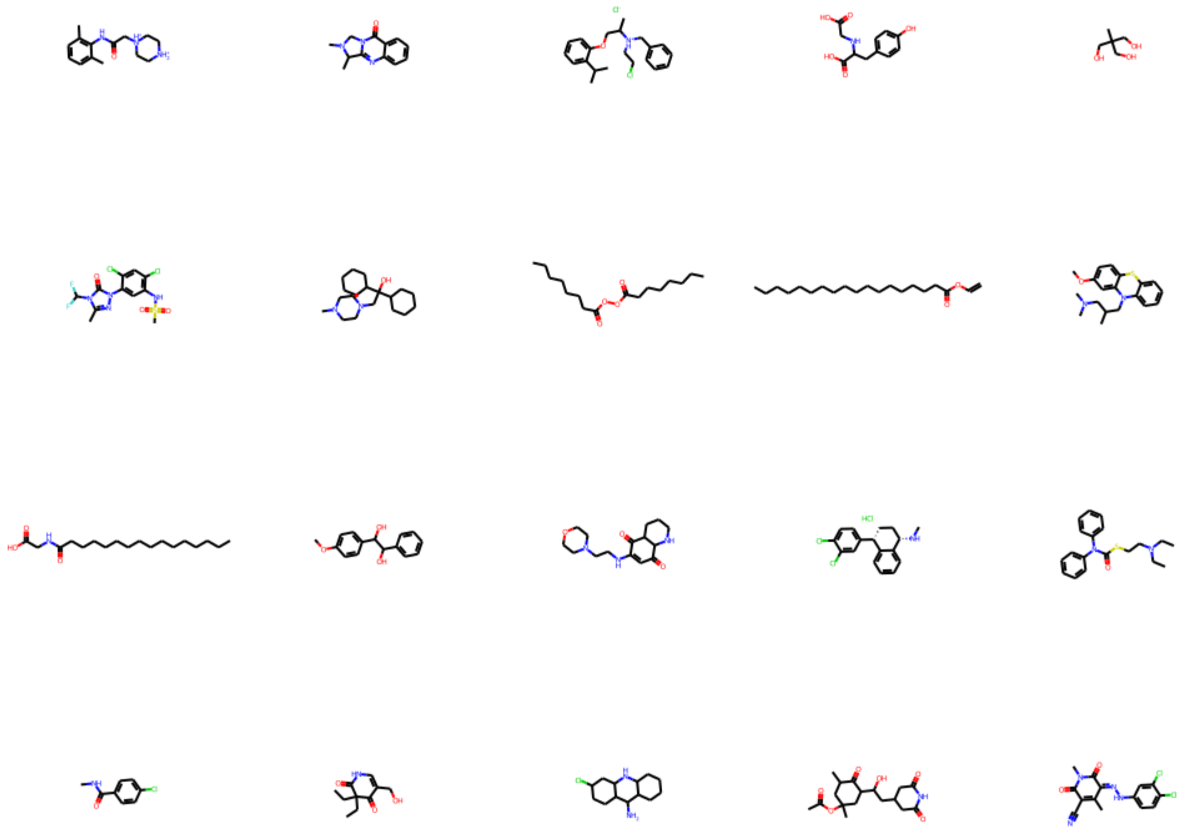

Figure S6: Examples of data outliers.

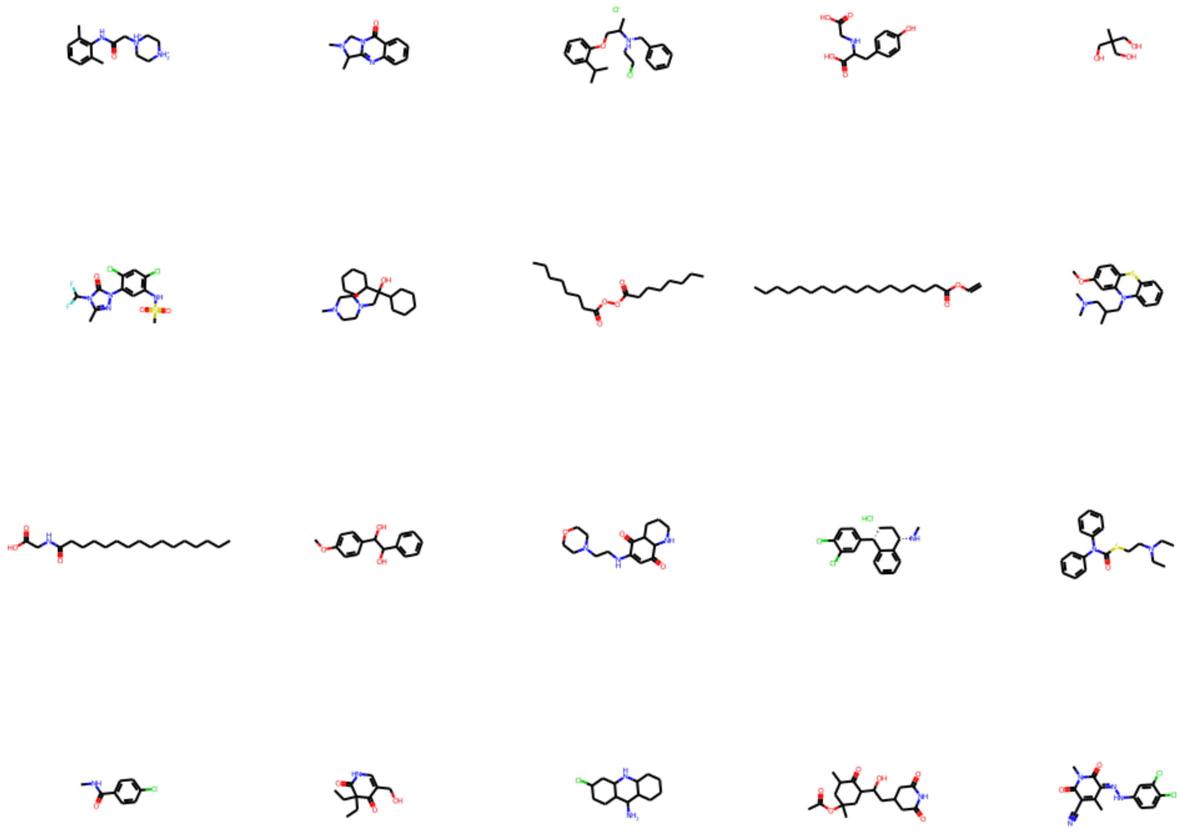

Figure S7: Examples of structural outliers.

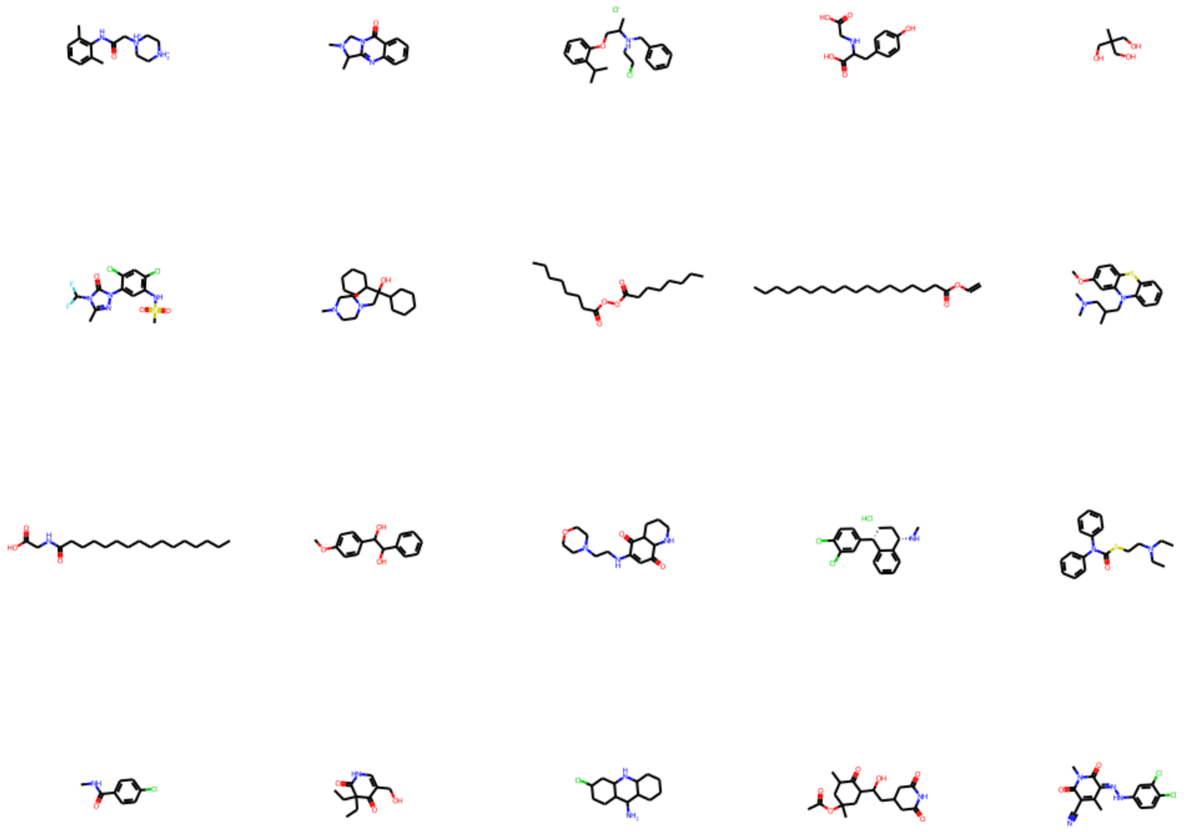

Figure S8: Examples of structural anomalies outliers.

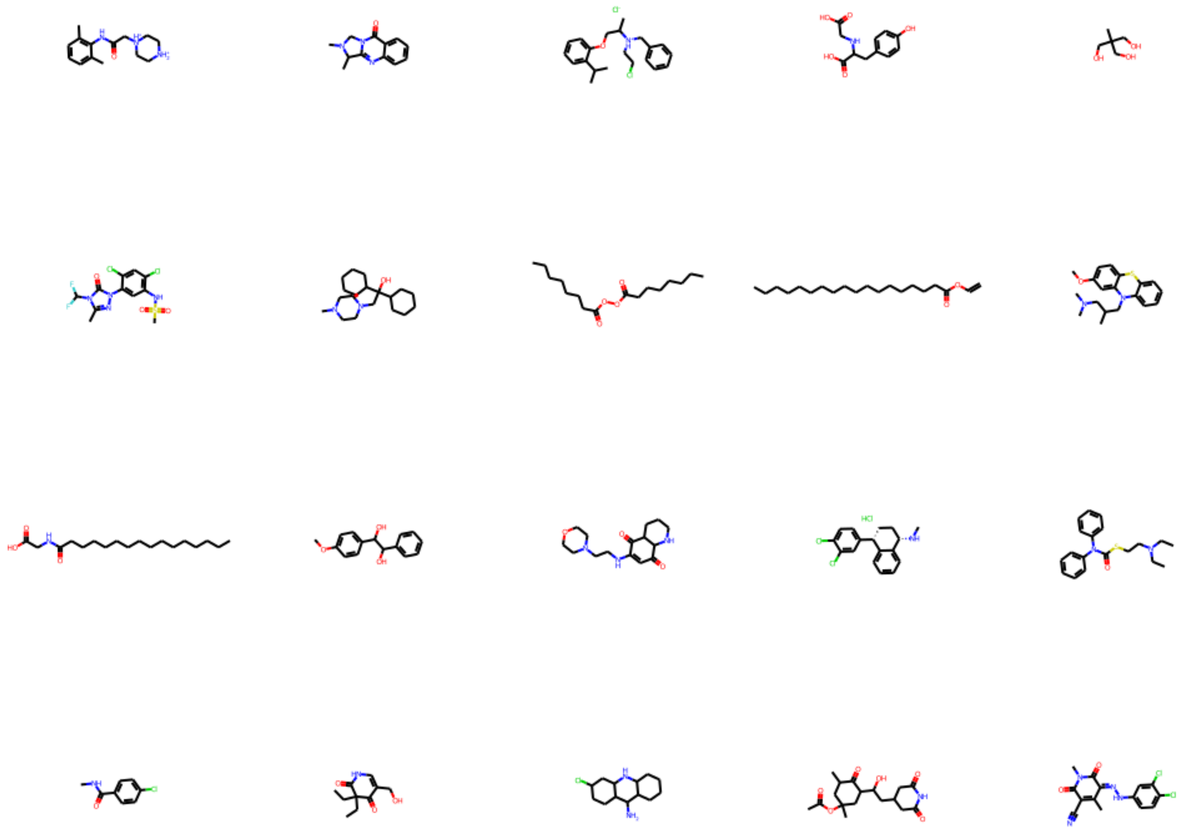

Figure S9: Examples of inliers.

# References


(1) Sorkun, M. C.; Khetan, A.; Er, S. AqSolDB, a curated reference set of aqueous solubility and 2D descriptors for a diverse set of compounds. *Scientific Data* **2019**, *6*, 143.

(2) Cui, Q.; Lu, S.; Ni, B.; Zeng, X.; Tan, Y.; Chen, Y. D.; Zhao, H. Improved Prediction of Aqueous Solubility of Novel Compounds by Going Deeper With Deep Learning. *Frontiers in Oncology* **2020**, *10*, 121.

(3) Moriwaki, H.; Tian, Y.-S.; Kawashita, N.; Takagi, T. Mordred: a molecular descriptor calculator. *Journal of Cheminformatics* **2018**, *10*, 4.

(4) Panapitiya, G.; Avendaño-Franco, G.; Ren, P.; Wen, X.; Li, Y.; Lewis, J. P. Machine-Learning Prediction of CO Adsorption in Thiolated, Ag-Alloyed Au Nanoclusters. *Journal of the American Chemical Society* **2018**, *140*, 17508–17514.
